# Supplementary material for: Adversarial Procedural Modeling: Learning Programs for Building Interiors
Source: arXiv:2611.40922 source file (2026-11-30)
Supplement: Supplementary file 1 [file supplement.tex]

% Separate supplement, one column (CVPR 2027 allows any legible format for supplementary PDFs).
% Anonymity: drop metadata of included figure PDFs (their creator tools, file names) from the output PDF.
\pdfsuppressptexinfo=-1
\documentclass[10pt,onecolumn,letterpaper]{article}
\usepackage[T1]{fontenc}
\usepackage[pagenumbers]{cvpr}
\input{preamble}
\usepackage{xr}\externaldocument{main}  % references to the main paper (e.g. Table 1)
\definecolor{cvprblue}{rgb}{0.21,0.49,0.74}
\usepackage[pagebackref,breaklinks,colorlinks,allcolors=cvprblue]{hyperref}
% Let floats sit next to the text that cites them, with little empty space around them.
\renewcommand{\topfraction}{0.95}\renewcommand{\bottomfraction}{0.9}\renewcommand{\textfraction}{0.05}
\renewcommand{\floatpagefraction}{0.85}\setcounter{topnumber}{4}\setcounter{bottomnumber}{4}\setcounter{totalnumber}{8}
\def\paperID{*****}
\def\confName{CVPR}
\def\confYear{2027}
\title{Adversarial Procedural Modeling:\\Learning Programs for Building Interiors}
\input{authors}
\author{\apmauthors}
\begin{document}
% One-column title block (cvpr.sty's \maketitlesupplementary forces two columns).
\begin{center}
  {\Large\textbf{\thetitle}}\\[0.5em]
  {\Large Supplementary Material}\\[1em]
  {\large\begin{tabular}[t]{c}\apmauthors\end{tabular}}
\end{center}
\vspace{1em}
% \maketitlesupplementary
\input{sec/X_suppl}
% \input{sec/supp_completeness}
{\small\bibliographystyle{ieeenat_fullname}\bibliography{main}}
\end{document}
